# Supplementary material for: Universalities of thermodynamic signatures in topological phases
Source: arXiv:1607.03373 source file (2016-12-15)
Supplement: Supplementary file 1 [file Supplementary_information_Universalities_of_thermodynamic_signatures_of_topological_phases.pdf]

# Universalities of thermodynamic signatures in topological phases
# Supplementary information

**S.N. Kempkes[1], A. Quelle[1], and Cristiane Morais Smith[1,*]**

[1]Institute for Theoretical Physics, Center for Extreme Matter and Emergent Phenomena, Utrecht University, Leuvenlaan 4, 3584 CE Utrecht, The Netherlands
[*]c.demoraissmith@uu.nl

August 31, 2016

## Results SSH model

The SSH model is a 1D model, which was first used to describe the dimerization of polyacetylene[1]. It describes electrons hopping between two neighboring sites of a bipartite lattice, and has proven to be an adequate tight-binding model for capturing the behavior of conjugated polymer chains. The SSH Hamiltonian reads

$$H_{\mathrm{SSH}} = \sum_n \left[ t_1 c^{\dagger}_{A,n} c_{B,n} + t_2 c^{\dagger}_{A,n+1} c_{B,n} + h.c. \right], \tag{1}$$

where $t_1$ and $t_2$ denote unequal hopping amplitudes between the even and odd links for the even (odd) sites $A$ ($B$). It is common to rewrite $t_1 = t(1+\Delta)$ and $t_2 = t(1-\Delta)$, which makes the Hamiltonian only dependent on the parameter $\Delta$, and thus there is a phase change between the topological and trivial phases for $\Delta = 0$. In Fig. 1, we show the results for the SSH chain for $t = 3/2$. We observe a first-order phase transition at the edge and a second-order phase transition in the bulk, which is precisely the same behavior obtained for the Kitaev chain.

Upon increasing the temperature, the phase transition smooths out. In Fig. 2 we compare the finite-$T$ phase diagram with the ones obtained via the Uhlmann phase, using the same procedure as for the Kitaev chain. Again, the comparison between the two results is clear.

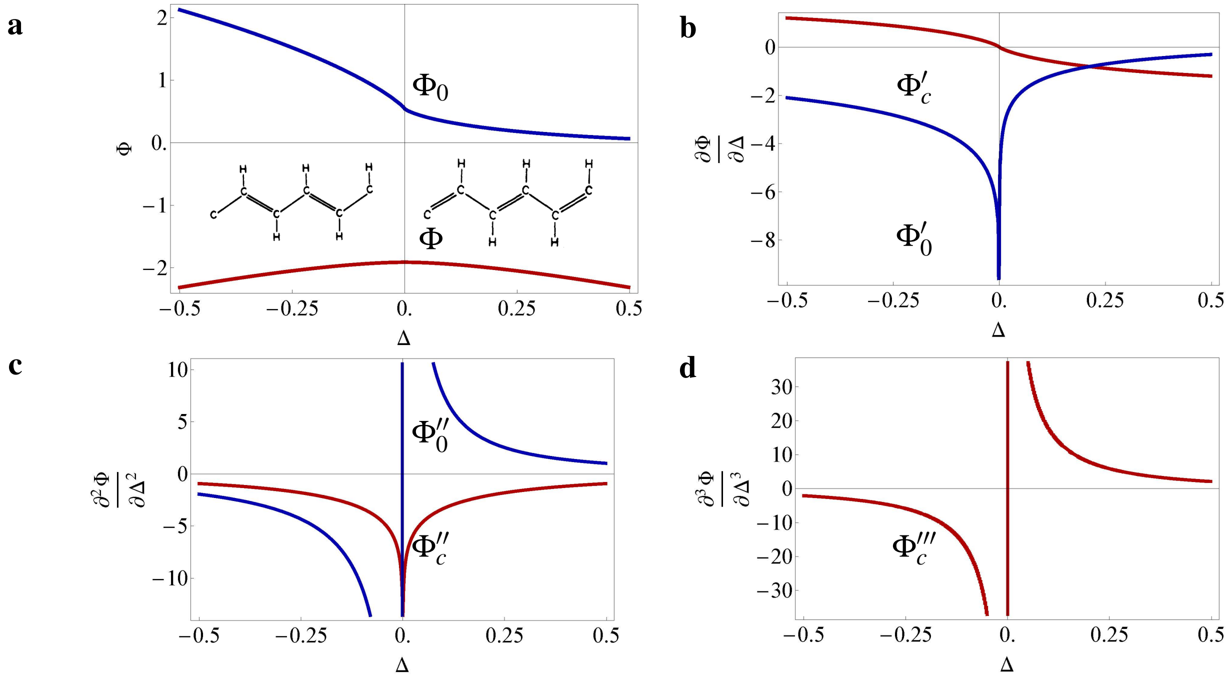


**Figure 1. Behavior of the thermodynamic potentials and their derivatives for the SSH model. a** The conventional potential $\Phi_c$ (red) and subdivision potential $\Phi_0$ (blue) and (**b, c, d**) their derivatives with respect to $\Delta$, for with $t = 3/2$. The figures show a similar behavior as the Kitaev chain, a first-order phase transition for the edge and a second-order phase transition in the bulk. The inset in **a** shows the topological (left) and trivial (right) phase of polyacetylene.

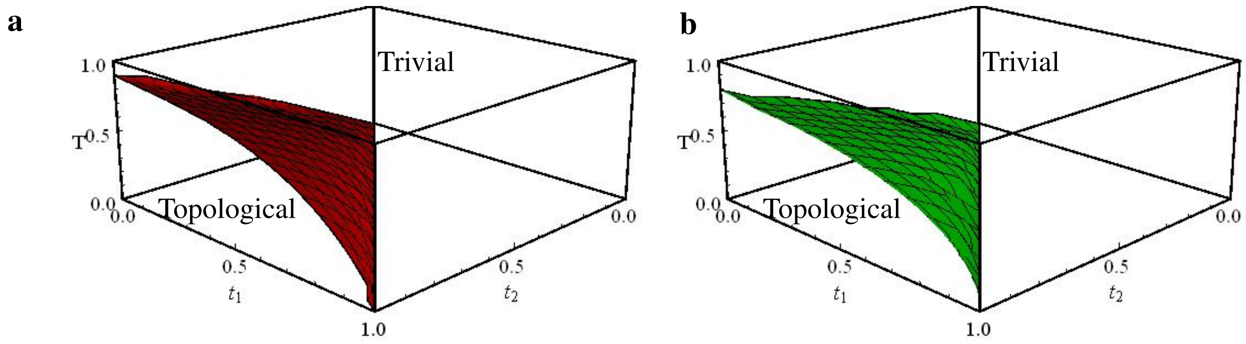


**Figure 2. Finite-$T$ phase diagram SSH model** The finite-$T$ phase diagram for the SSH model obtained via **a** Hill thermodynamics (red) and **b** via the Uhlmann phase (green)[2].

# References


1. Su, W. P., Schrieffer, J. R. & Heeger, A. J. Solitons in polyacetylene. *Phys. Rev. Lett.* **42**, 1698–1701 (1979).

2. Viyuela, O., Rivas A. & Martin-Delgado, M. A., Uhlmann Phase as a Topological Measure for One-Dimensional Fermion Systems. *Physical Review Letters* **112**, 130401(2014).
